# Supplementary material for: Maximum Weight Online Matching with Deadlines
Source: arXiv:1808.03526 source file (2018-08-09)
Supplement: Supplementary file 1 [file appendix_ro.tex]

\appendix
\addcontentsline{toc}{chapter}{APPENDICES}
\begin{conjecture}
  $\alpha'_d$ is decreasing in $d$.
\end{conjecture}

\subsection{Warm-up: factor $3$ for $d = 3$}
\label{sec:warm_up}

Let $n$ be a multiple of $8$,
Based on Lemma \ref{lem:cover}, it is enough to find three permutations of $S_n$ such that every edge in $G(id)$ is in at least one of the permutations.

Note that in the realized graph $G(id)$, every vertex $i \in [3, n-3]$ is connected to exactly $i-1, i-2, i-3, i+1, i+2, i+3$

Bellow we show how we can cover every edge in $G(id)$ with edges in $G'(\sigma_1), G'(\sigma_2), G'(\sigma_3)$ for $\sigma_1, \sigma_2, \sigma_3$ three periodic permutations.

\begin{table}[h!]
\begin{tabular}{ l |l |l |l |l |l |l |l  }
 & 2, 3, 4, 5 & 6, 7, 8, 9 & 10, 11, 12, 13 & 14, 15, 16, 17 & 18, 19, 20, 21 & 22, 23, 24, 25 & ... \\
 & 0, 1, 2, 4 & 3, 5, 6, 7 & 8, 9, 10, 12 & 11, 13, 14, 15 & 16, 17, 18, 20 & 19, 21, 22, 23  & ... \\
 & 4, 6, 7, 10 & 5, 8, 9, 11 & 12, 14, 15, 18 & 13, 16, 17, 19 & 20, 22, 23, 26 & 21, 24, 25, 27  & ... \\
\end{tabular}

\caption{3-covering of the cycle to the power $3$ with $8$-periodic permutations which induce $4$-cliques. Vertical lines correspond to the batching cuts (e.g under the bottom permutation, vertices 4,6,7,10 will be in the same clique.)}
\end{table}

\mb{Need to take care of edge cases better.}

\subsection{Factor $4$ for any $d$ multiple of $2$.}
\label{sec:factor4}

The idea is that when $d$ is a multiple of $2$, we can split vertices into groups of size $d/2$. We will consider each groups to be a vertex in a graph $\widetilde{G}$, with an edge between two groups $a$ and $b$ if there exist two vertices $i \in a$ and $j \in b$ with an edge $(i,j)$ in the original graph $G(id)$.

Observe that the graph $\widetilde{G}$ is itself a cycle to the power $2$.
We wish to cover this cycle with clique-graphs $G'_2(\sigma)$.
Note that the covering in section \ref{sec:warm_up} is made easier by the fact that the clique size is allowed to be $d+1$ even though each vertex is connected to "only" $d$ vertices before and after.

Suppose that we have a 4-cover over edges in $\widetilde{G}$, one can recover a 4-cover over edges in the original graph $G(id)$ by simply replacing each group with the vertices that it contains.

\begin{table}[h!]
  \centering
  \begin{tabular}{ l |l |l |l |l |l |l |l }
    0, 1 & 2, 3 & 4, 5 & 6, 7 & 8, 9 & 10, 11 & 12, 13 & 14, 15 \\
    0, 2 & 1, 3 & 4, 6 & 5, 7 & 8, 10 & 9, 11 & 12, 14 & 13, 15 \\
    2, 4 & 3, 5 & 6, 8 & 7, 9 & 10, 12 & 11, 13 & 14, 0 & 15, 1 \\
    1, 2 & 3, 4 & 5, 6 & 7, 8 & 9, 10 & 11, 12 & 13, 14 & 15, 0 \\
  \end{tabular}

\caption{4-covering of the cycle to the power $2$ with $4$-periodic permutations which induce $2$-cliques.}
\end{table}

\subsection{Main result: factor $3.5$ for $d$ multiple of $3$}

The idea is to generalize the result from section \ref{sec:factor4} by separating vertices into $3$ groups. We also find a fractional cover: each permutation will receive a coefficient $0.5$. Therefore, each edge needs to be covered by at least two permutations.

\begin{table}[h!]
  \centering
  \begin{tabular}{ l |l |l |l |l |l |l |l }
  1, 2, 3 & 4, 5, 6 & 7, 8, 9 & 10, 11, 12 & 13, 14, 15 & 16, 17, 18 & 19, 20, 21 & 22, 23, 0 \\
  3, 4, 6 & 5, 7, 8 & 9, 10, 12 & 11, 13, 14 & 15, 16, 18 & 17, 19, 20 & 21, 22, 0 & 23, 1, 2 \\
  0, 1, 4 & 2, 3, 5 & 6, 7, 10 & 8, 9, 11 & 12, 13, 16 & 14, 15, 17 & 18, 19, 22 & 20, 21, 23 \\
  3, 4, 7 & 5, 6, 8 & 9, 10, 13 & 11, 12, 14 & 15, 16, 19 & 17, 18, 20 & 21, 22, 1 & 23, 0, 2 \\
  0, 3, 5 & 1, 2, 4 & 6, 9, 11 & 7, 8, 10 & 12, 15, 17 & 13, 14, 16 & 18, 21, 23 & 19, 20, 22 \\
  3, 6, 8 & 4, 5, 7 & 9, 12, 14 & 10, 11, 13 & 15, 18, 20 & 16, 17, 19 & 21, 0, 2 & 22, 23, 1 \\
  0, 1, 3 & 2, 4, 5 & 6, 7, 9 & 8, 10, 11 & 12, 13, 15 & 14, 16, 17 & 18, 19, 21 & 20, 22, 23 \\
  \end{tabular}

\caption{$3.5$-covering of the cycle to the power $3$ with $6$-periodic permutations which induce $3$-cliques.}
\end{table}

\section{Methodology}
Denote $P_n^d$ the set of $2d$-periodic permutations over $n$ vertices.
The above permutations can be found by solving the following Linear Program:
\mb{TODO}
% \begin{equation}
%   \begin{split}
%      \min & \alpha \\
%      &\text{s.t. } \sum_{\sigma_i \in P_n^d}

\section{Going further: factor $3.152$ for $d$ multiple of $5$}

\begin{table}[h!]
  \centering
  \begin{tabular}{ l |l |l |l |l |l }
  2, 3, 4, 5, 6 & 7, 8, 9, 10, 11 & 12, 13, 14, 15, 16 & 17, 18, 19, 20, 21 & 22, 23, 24, 25, 26 & 27, 28, 29, 0, 1 \\
  2, 3, 4, 5, 7 & 6, 8, 9, 10, 11 & 12, 13, 14, 15, 17 & 16, 18, 19, 20, 21 & 22, 23, 24, 25, 27 & 26, 28, 29, 0, 1 \\
  3, 4, 5, 6, 10 & 7, 8, 9, 11, 12 & 13, 14, 15, 16, 20 & 17, 18, 19, 21, 22 & 23, 24, 25, 26, 0 & 27, 28, 29, 1, 2 \\
  4, 5, 6, 7, 11 & 8, 9, 10, 12, 13 & 14, 15, 16, 17, 21 & 18, 19, 20, 22, 23 & 24, 25, 26, 27, 1 & 28, 29, 0, 2, 3 \\
  1, 2, 3, 5, 6 & 4, 7, 8, 9, 10 & 11, 12, 13, 15, 16 & 14, 17, 18, 19, 20 & 21, 22, 23, 25, 26 & 24, 27, 28, 29, 0 \\
  0, 1, 2, 5, 7 & 3, 4, 6, 8, 9 & 10, 11, 12, 15, 17 & 13, 14, 16, 18, 19 & 20, 21, 22, 25, 27 & 23, 24, 26, 28, 29 \\
  2, 3, 5, 6, 7 & 4, 8, 9, 10, 11 & 12, 13, 15, 16, 17 & 14, 18, 19, 20, 21 & 22, 23, 25, 26, 27 & 24, 28, 29, 0, 1 \\
  5, 6, 8, 10, 11 & 7, 9, 12, 13, 14 & 15, 16, 18, 20, 21 & 17, 19, 22, 23, 24 & 25, 26, 28, 0, 1 & 27, 29, 2, 3, 4 \\
  5, 6, 8, 10, 13 & 7, 9, 11, 12, 14 & 15, 16, 18, 20, 23 & 17, 19, 21, 22, 24 & 25, 26, 28, 0, 3 & 27, 29, 1, 2, 4 \\
  1, 2, 5, 6, 9 & 3, 4, 7, 8, 10 & 11, 12, 15, 16, 19 & 13, 14, 17, 18, 20 & 21, 22, 25, 26, 29 & 23, 24, 27, 28, 0 \\
  5, 7, 8, 12, 13 & 6, 9, 10, 11, 14 & 15, 17, 18, 22, 23 & 16, 19, 20, 21, 24 & 25, 27, 28, 2, 3 & 26, 29, 0, 1, 4 \\
  0, 2, 4, 7, 9 & 1, 3, 5, 6, 8 & 10, 12, 14, 17, 19 & 11, 13, 15, 16, 18 & 20, 22, 24, 27, 29 & 21, 23, 25, 26, 28 \\
  0, 2, 5, 7, 9 & 1, 3, 4, 6, 8 & 10, 12, 15, 17, 19 & 11, 13, 14, 16, 18 & 20, 22, 25, 27, 29 & 21, 23, 24, 26, 28 \\
  5, 7, 10, 12, 14 & 6, 8, 9, 11, 13 & 15, 17, 20, 22, 24 & 16, 18, 19, 21, 23 & 25, 27, 0, 2, 4 & 26, 28, 29, 1, 3 \\
  0, 3, 4, 7, 8 & 1, 2, 5, 6, 9 & 10, 13, 14, 17, 18 & 11, 12, 15, 16, 19 & 20, 23, 24, 27, 28 & 21, 22, 25, 26, 29 \\
  5, 9, 10, 12, 14 & 6, 7, 8, 11, 13 & 15, 19, 20, 22, 24 & 16, 17, 18, 21, 23 & 25, 29, 0, 2, 4 & 26, 27, 28, 1, 3 \\
  5, 9, 10, 13, 14 & 6, 7, 8, 11, 12 & 15, 19, 20, 23, 24 & 16, 17, 18, 21, 22 & 25, 29, 0, 3, 4 & 26, 27, 28, 1, 2 \\
  5, 8, 9, 13, 14 & 6, 7, 10, 11, 12 & 15, 18, 19, 23, 24 & 16, 17, 20, 21, 22 & 25, 28, 29, 3, 4 & 26, 27, 0, 1, 2 \\
  5, 8, 9, 11, 13 & 6, 7, 10, 12, 14 & 15, 18, 19, 21, 23 & 16, 17, 20, 22, 24 & 25, 28, 29, 1, 3 & 26, 27, 0, 2, 4 \\
  0, 3, 4, 5, 8 & 1, 2, 6, 7, 9 & 10, 13, 14, 15, 18 & 11, 12, 16, 17, 19 & 20, 23, 24, 25, 28 & 21, 22, 26, 27, 29 \\
  5, 7, 9, 12, 14 & 6, 8, 10, 11, 13 & 15, 17, 19, 22, 24 & 16, 18, 20, 21, 23 & 25, 27, 29, 2, 4 & 26, 28, 0, 1, 3 \\
  0, 2, 4, 5, 9 & 1, 3, 6, 7, 8 & 10, 12, 14, 15, 19 & 11, 13, 16, 17, 18 & 20, 22, 24, 25, 29 & 21, 23, 26, 27, 28 \\
  4, 6, 7, 10, 11 & 5, 8, 9, 12, 13 & 14, 16, 17, 20, 21 & 15, 18, 19, 22, 23 & 24, 26, 27, 0, 1 & 25, 28, 29, 2, 3 \\
  0, 2, 3, 5, 7 & 1, 4, 6, 8, 9 & 10, 12, 13, 15, 17 & 11, 14, 16, 18, 19 & 20, 22, 23, 25, 27 & 21, 24, 26, 28, 29 \\
  5, 7, 8, 10, 12 & 6, 9, 11, 13, 14 & 15, 17, 18, 20, 22 & 16, 19, 21, 23, 24 & 25, 27, 28, 0, 2 & 26, 29, 1, 3, 4 \\
  0, 1, 5, 6, 9 & 2, 3, 4, 7, 8 & 10, 11, 15, 16, 19 & 12, 13, 14, 17, 18 & 20, 21, 25, 26, 29 & 22, 23, 24, 27, 28 \\
  0, 1, 4, 5, 9 & 2, 3, 6, 7, 8 & 10, 11, 14, 15, 19 & 12, 13, 16, 17, 18 & 20, 21, 24, 25, 29 & 22, 23, 26, 27, 28 \\
  0, 1, 4, 5, 6 & 2, 3, 7, 8, 9 & 10, 11, 14, 15, 16 & 12, 13, 17, 18, 19 & 20, 21, 24, 25, 26 & 22, 23, 27, 28, 29 \\
  5, 6, 8, 11, 13 & 7, 9, 10, 12, 14 & 15, 16, 18, 21, 23 & 17, 19, 20, 22, 24 & 25, 26, 28, 1, 3 & 27, 29, 0, 2, 4 \\
  0, 1, 3, 5, 8 & 2, 4, 6, 7, 9 & 10, 11, 13, 15, 18 & 12, 14, 16, 17, 19 & 20, 21, 23, 25, 28 & 22, 24, 26, 27, 29 \\
  1, 2, 4, 5, 6 & 3, 7, 8, 9, 10 & 11, 12, 14, 15, 16 & 13, 17, 18, 19, 20 & 21, 22, 24, 25, 26 & 23, 27, 28, 29, 0 \\
  0, 1, 2, 5, 6 & 3, 4, 7, 8, 9 & 10, 11, 12, 15, 16 & 13, 14, 17, 18, 19 & 20, 21, 22, 25, 26 & 23, 24, 27, 28, 29 \\
  5, 6, 7, 10, 11 & 8, 9, 12, 13, 14 & 15, 16, 17, 20, 21 & 18, 19, 22, 23, 24 & 25, 26, 27, 0, 1 & 28, 29, 2, 3, 4 \\
  0, 1, 2, 4, 5 & 3, 6, 7, 8, 9 & 10, 11, 12, 14, 15 & 13, 16, 17, 18, 19 & 20, 21, 22, 24, 25 & 23, 26, 27, 28, 29 \\
  4, 5, 6, 7, 10 & 8, 9, 11, 12, 13 & 14, 15, 16, 17, 20 & 18, 19, 21, 22, 23 & 24, 25, 26, 27, 0 & 28, 29, 1, 2, 3 \\
  5, 6, 7, 8, 11 & 9, 10, 12, 13, 14 & 15, 16, 17, 18, 21 & 19, 20, 22, 23, 24 & 25, 26, 27, 28, 1 & 29, 0, 2, 3, 4 \\
  3, 4, 5, 6, 8 & 7, 9, 10, 11, 12 & 13, 14, 15, 16, 18 & 17, 19, 20, 21, 22 & 23, 24, 25, 26, 28 & 27, 29, 0, 1, 2 \\
\end{tabular}
\caption{$3.152$-covering of the cycle to the power $5$ with $10$-periodic permutations which induce $5$-cliques. The coefficients associated with this covering are $0.0275804, 0.00867133, 0.156531, 0.103273, 0.228867, 0.00027972, 0.14014, 0.0338182, 0.17765, 0.11642$, $0.12372, 0.0298182, 0.078042, 0.0218462, 0.0113846, 0.0375385, 0.177762, 0.118685, 0.0160559, 0.0915804$, $0.0318042, 0.0591329, 0.0438601, 0.18386, 0.10565, 0.116783, 0.192531, 0.0254545, 0.0363636, 0.132839$, $0.0261259, 0.0325315, 0.0671608, 0.086965, 0.222042, 0.0898462, 0.000111888$.}
\end{table}

%
% $$\E[\off] \leq 4 \E[\bat].$$
